# Supplementary material for: Motility Modulates the Partitioning of Bacteria in Aqueous Two-Phase Systems
Source: arXiv:2405.08995 ancillary file (2024-12-20)
Supplement: Supplementary file 1 [file Supporting_information.pdf]

# Motility Modulates the Partitioning of Bacteria in Aqueous Two-Phase Systems

Jiyong Cheon,[1] Kyu Hwan Choi,[2] Kevin J. Modica,[2] Robert J. Mitchell,[3] Sho C. Takatori,[2,*] and Joonwoo Jeong[1,†]

[1] *Department of Physics, Ulsan National Institute of Science and Technology, Ulsan, Republic of Korea*
[2] *Department of Chemical Engineering, University of California, Santa Barbara, Santa Barbara, CA, USA*
[3] *Department of Biological Sciences, Ulsan National Institute of Science and Technology, Ulsan, Republic of Korea*

(Dated: December 20, 2024)

## I Description of Supplementary Movies

**Movie S1:** Motile *Bacillus subtilis* dispersed in the ATPS (dextran concentration: 3.2 wt/wt% and PEG concentration: 2.5 wt/wt%). All bacteria in this large field of view are in focus, suggesting that this is a quasi-2D system. Scale bar = 50 $\mu$m
**Movie S2:** Optical tweezers-guided crossing of a silica bead-bound bacterium across the interface. Scale bar = 20 $\mu$m.
**Movie S3:** Motile *Bacillus subtilis* dispersed in the ATPS (dextran concentration: 8.0 wt/wt% and PEG concentration: 2.5 wt/wt%). Scale bar = 50 $\mu$m
**Movie S4:** Motile *Bacillus subtilis* crosses the interface of ATPS (dextran concentration: 3.2 wt/wt% and PEG concentration: 2.5 wt/wt%). Scale bar = 10 $\mu$m

* stakatori@ucsb.edu
† jjeong@unist.ac.kr

## II Experimental Methods

### A Bacterial cell culture

For the partitioning-ratio measurements, mid-exponentially growing *Bacillus subtilis* strain ATCC 6051 was used. For this, bacterial colonies were first cultured overnight on a lysogeny broth (Duchefa Biochemie, Netherlands) agar plate at 37°C. A single colony was transferred into sterile terrific broth (TB; MBcell, Republic of Korea) and cultured in a shaking chamber (250 rpm) at 37°C. After overnight growth, an aliquot of the bacterial culture was transferred to fresh TB (optical density (O.D. at 600 nm) = 0.03) and cultured under the same condition for 2.5 hours (O.D. ∼ 0.5 at 600 nm). At this point, the bacteria were pelleted and resuspended in a sterile M9 minimal medium (MBcell, Republic of Korea) to prevent further division.

*Optical tweezers experiment.* For the optical tweezers experiments, a single colony of *Bacillus subtilis* strain ATCC 6051, grown as described above, was inoculated into 2 ml of TB, and cultured in a shaking incubator (100 rpm) at 37°C. After overnight growth, an aliquot of the bacterial culture was transferred to fresh TB (1:10 dilution) and cultured under the same condition for ∼4 hours. 2 ml of bacterial suspension was then pelleted (6k RCF for 1 min) and washed in deionized water. This wash step was repeated five times before the cells were resuspended in 400$\mu$L of deionized water.

### B Sample preparation

We utilized two different polymers: PEG (Polyethylene Glycol) with a molecular weight of 35,000 Da from Sigma-Aldrich (USA), and dextran with a molecular weight of 500,000 Da from Spectrum (USA), to create an Aqueous Two-Phase System (ATPS). Both polymers were dissolved in M9 (for partitioning ratio measurement) or deionized water (for optical tweezers experiment) to measure the partitioning ratio and force, respectively. The dextran concentrations were systematically adjusted to achieve final concentrations (including bacteria) of 1.5, 2.5, 3.2, 4, 5, and 8% (wt/wt), while the PEG concentration was maintained at 2.5%. The final bacterial densities were adjusted to an O.D. of 1 (partitioning ratio measurement) or 0.05 (force measurement) by pelleting the bacteria at 8k RCF for 1 min and resuspending them in an appropriate volume of either M9 or deionized water.

The quasi-2D cell gap was controlled by the volume of the bacterial ATPS solution. For example, to measure the partitioning ratio of bacteria, a $\sim 1.3\mu$L volume of the bacterial ATPS solution is sandwiched between a polymeric, air-permeable coverslip (SPL Life Science, Republic of Korea). Based on the area of the coverslip (254 mm$^2$, 9 mm diameter), the cell gap was estimated to be $\ll 5\mu$m with the two phases to be horizontally separated by an interface. In the optical tweezers experiment, we used a 25×25 mm$^2$ coverslip where the cell gap was $\ll 5\mu$m.

A confocal image, taken with a Leica SP8 Resonant Scanning Confocal microscope using a solution containing dissolved Alexa Fluor 647-labeled dextran (40,000 Da) in a 3.2 wt/wt% dextran and 2.5 wt/wt% PEG ATPS solution, confirmed that a wall-like interface formed between and separated these two phases completely.

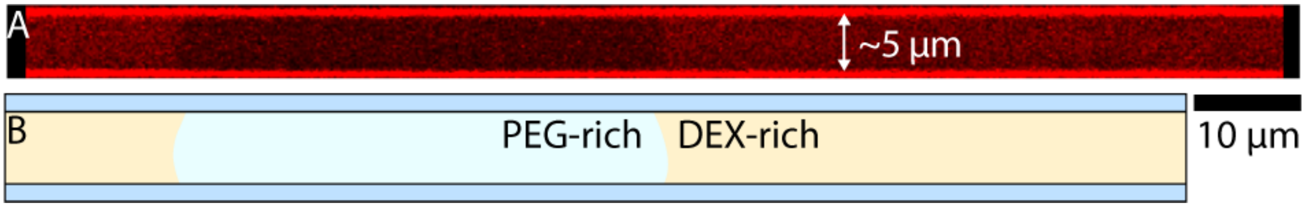


FIG. S1. Configuration of the observation cell. A) Confocal image of the sandwich cell with labeled dextran and B) schematic image of the cell. The dark region of Panel A is the PEG-rich phase, and the red region represents the Alexa Fluor 647-labeled DEX-rich phase. The cell thickness is ∼ 5$\mu$m, and the 10-$\mu$m scale bar only applies to the lateral direction.

### C Motility suppression of *B. subtilis*

For the non-motile controls, the *B. subtilis* suspensions were incubated at 65°C for 10 minutes.

## III Partitioning ratio measurement

### A Observation

The samples were observed using an inverted phase-contrast microscope (BX53-P; Olympus) at room temperature (23 °C). Image stacks, spanning up to 20 hours, were captured at the rate of 1 frame per second using a 20× dry objective and a CCD camera (INFINITY5-3M; Lumenera). We used a green illumination derived from an LED lamp (U-LEDPS; Olympus) equipped with a 550-nm filter (43IF550-W45; Olympus).

### B Methods and result

We chose a domain of the PEG-rich phase enclosed by the DEX-rich phase within the image stacks and adjusted the view so that this PEG-rich island was located at the center of the image, making the area of each phase equal, as shown in Fig. S2. Then we counted the number of bacteria inside and outside of the PEG-rich domain, as shown in Fig. S3A, until the partitioning ratio reached a steady-state, as shown in Fig. S3B.

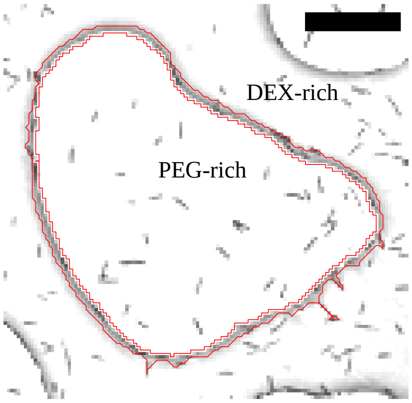


FIG. S2. Experimental image of the sampled area. The PEG-rich island was adjusted to be at the center. The red lines highlights the interface. The number of bacteria inside and outside of the PEG-rich island was then counted. Scale bar = 50$\mu$m

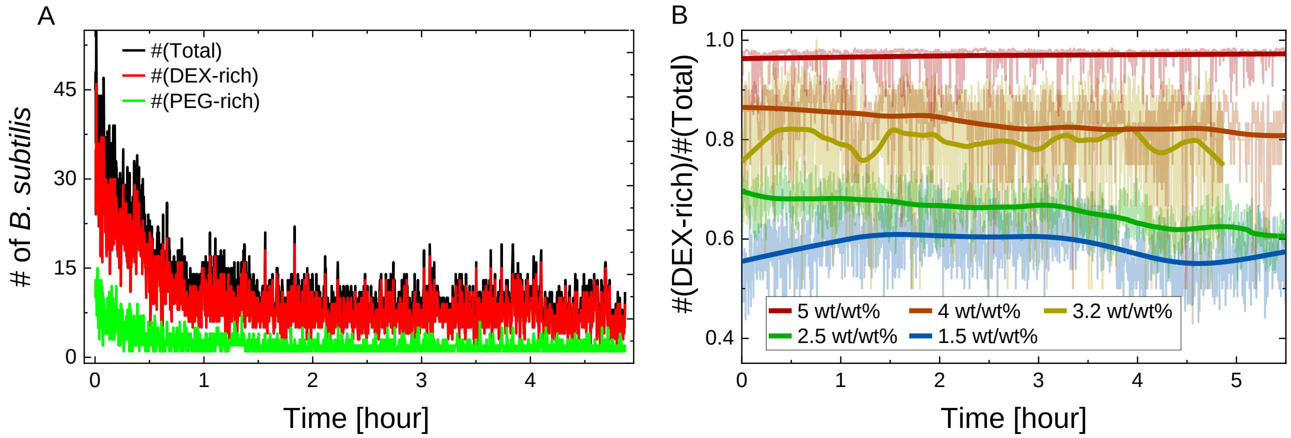


FIG. S3. Change in the number and partitioning ratio of bacteria in sampled areas over time. (A) The number of bacteria inside(green) and outside(red) of the sampled PEG-domain and the total(black) are plotted. Approaching the steady state, the total number may decrease or increase according to regions because the initial distribution after the cell preparation is not uniform. (B) Steady-state partitioning ratio, with each color indicating the concentration of dextran employed in each test. The thick solid lines after smoothing illustrate the partitioning trend over time. The raw data plotted here were used to calculate the values in Fig.2.

## IV Rule out the chemotaxis

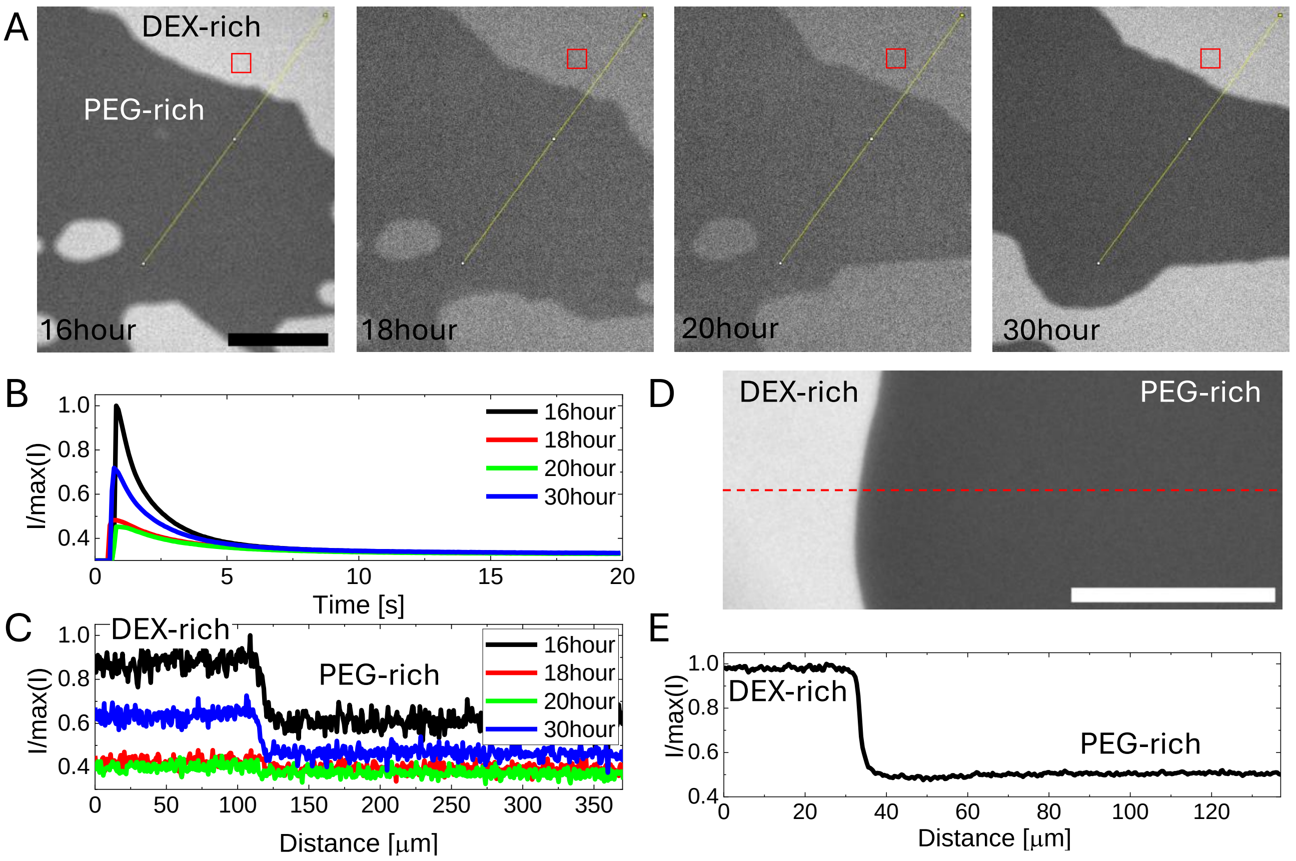


FIG. S4. Fluorescence microscope image of ATPS and its normalized intensity profile. (A) The phase-separated system and its fluorescence signal images were obtained 16, 18, 20, and 30 hours after the cell assembly of the solution containing 3.2 wt/wt% of DEX, 2.5 wt/wt% of PEG, and 0.0004 wt/wt% of DEX-FITC. (B) The normalized intensity profile in the red box at the DEX-rich phase corresponds with the measuring time where the maximum intensity from 16 hours' measurements was used as max(I) as a normalizing constant. The normalized intensity profile of the yellow line of (A), which corresponds with the dextran composition, is plotted in (C). (D) The phase-separated system and its fluorescence signal images in higher magnification. The normalized intensity profile of the red line of (D), which corresponds with the dextran composition, is plotted in (E). Scale bar = 50 $\mu$m

The fluorescent DEX-FITC is added in the ATPS and condensed in the DEX-rich phases, as shown in Fig. S4(A and D). Fig. S4(A) shows a fluorescence image sequence of a fixed field of view at 16, 18, 20, and 30 hours after the sample assembly. It demonstrates the diffusion-induced fluorescence recovery after photo-bleaching, of which the fluorescence signal from the red box in Fig. S4(A) during the 20-sec bleaching is shown in Fig. S4(B). As shown in Fig. S4(C), the decay of the DEX-FITC fluorescence signal across the interface is short-ranged, regardless of the time. This observation indicates that the DEX concentration gradient after equilibration is short-ranged, disputing the chemotaxis scenario. Figure S4(D and E) with a higher magnification depicts the gradient as narrow as 2 $\mu$m.

## V Attaching optical tweezers handle to the bacteria

We attached a spherical silica bead as a handle on the bacterium's surface to calibrate the force in the optical tweezers experiment. Grabbing the handle on the bacterium rather than the bacterial body with the optical tweezers simplifies the force calculation by reducing any complexity arising from an anisotropic morphology of the bacterium, as well as changes in the refractive index while crossing the PEG-dextran interface.

Attaching a handle to the bacteria was achieved in two steps. Partially oxidizing the bacterial surface is the first. The second is a biotinylation process involving hydrazide biotin (Thermo Fisher Scientific). During the first step, the surfaces of the bacteria are partially oxidized and treated by adding 20 $\mu$l of aqueous 100 mM $NaIO_4$ (Sigma-Aldrich) solution into 100 $\mu$l of the washed bacterial solution. After 30 min at room temperature, 22 °C, the bacteria were pelleted (6k RCF for 1min) and washed 5 times with deionized water. Then the sedimented pellet is dispersed into 50 $\mu$l of deionized water for the biotinylation step. To chemically bind biotin to the bacterial surface, aqueous solutions of 10 $\mu$l of 100 mM aniline (Sigma-Aldrich) and 10 $\mu$l of 100 mM hydrazide biotin were added to the partially oxidized bacteria solution (50 $\mu$l) to make a final concentration of 14.3 mM of aniline and 14.3 mM of a binding material. This was incubated at 36℃ for 2 hours, after which the oxidation reaction was quenched by adding 1 mL of deionized water. The biotinylated bacterial cells were collected into 50 $\mu$l of deionized water after five rounds of pelleting (6k RCF for 1 min) and washing with deionized water.

Streptavidin-functionalized silica beads (SA-bead, 3-3.9 $\mu$m, Spherotech) were added to the biotinylated bacteria suspension. For this, 5 $\mu$l of biotinylated bacterial cells and 5 $\mu$l of 0.5 wt/wt% SA-bead solution in deionized water were mixed with 200 $\mu$l of the ATPS solution. The biotin present on the bacterial surface is bound by the streptavidin on the particle to form a strong bond.

## VI Optical tweezers measurement

### A Observation and method

An inverted microscope(TI-2 Eclipse, Nikon) with 100x objective lens (CFI Plan Apo lambda) was used. The optical trapping was controlled by Tweez300 software (Aresis). In this study, the laser beam grasped the spherical handle attached to the bacterial surface and dragged the bacterium across the interface. The dragging velocity was maintained at a value of $0.5-2$ $\mu$m/s, which is slow enough to neglect the viscous drag ($6\pi\eta rv : 0.10 \sim 0.41$pN where $r = 1$ $\mu$m, $\eta = 11$ mPa $\cdot$ s and $v = 0.5 - 2$ $\mu$m/s) when compared to the force applied by the interface ($\gg$ 1pN). Namely, as the laser beam moved, the sphere remained at the laser beam's focal point, and any displacement observed should result from external forces, specifically those from the interface. As the bacterium moved, we tracked the spherical handle and compared its position against the position of the laser focal point, which moved at a constant speed. The difference between these two positions is defined as d$x$, where the force applied on the particle ($F$) is defined as $F = \kappa_{\rm t} \cdot {\rm d}x$, with trap stiffness, $\kappa_{\rm t}$, listed in Table. I.

### B Trap stiffness

The trap stiffness ($\kappa_{\rm t}$) for the force measurement was determined from the analysis of a Brownian particle trapped with different laser powers. Because of the parabolic shape of the potential in the vicinity of the trapping focus, the particle's displacement from the laser focus follows a Gaussian probability distribution, represented as $P(dr) = \frac{1}{\sigma\sqrt{2\pi}}e^{-\frac{1}{2}\left(\frac{dr}{\sigma}\right)^2}$, where $dr$ represents the displacement from the focus and $\sigma$ is the standard deviation. The exponent in this expression corresponds to the dimensionless trapping energy, given by $\frac{E_{\rm trap}}{k_{\rm B}T} = -\frac{1}{2}\frac{\kappa_t dr^2}{k_{\rm B}T}$, where $k_{\rm B}$ is the Boltzmann constant, and $T$ is the temperature of the system. Thus, experimental measurement of $\sigma^2$ can determine $\kappa_t = \frac{k_{\rm B}T}{\sigma^2}$.

Trap stiffnesses were measured with more than five different laser powers in the range 2 - 15% of the maximum laser power. Then, a linear regression line depending on laser powers can estimate the trap stiffness at an experimental power range of 10-80% of the maximum laser power using extrapolation.

| Dextran concentration [wt/wt%] | 1.5 | 2.5 | 3.2 | 4 | 5 | 8 |
|---|---|---|---|---|---|---|
| Slope [pN/$\mu$m/% of $P_{\rm max}$] | 8.78 | 9.82 | 9.57 | 8.86 | 6.91 | 8.08 |

TABLE I. Slope from the linear regression relating the trap stiffness to the percentage of the maximum laser power.

## VII Effects of interface deformation

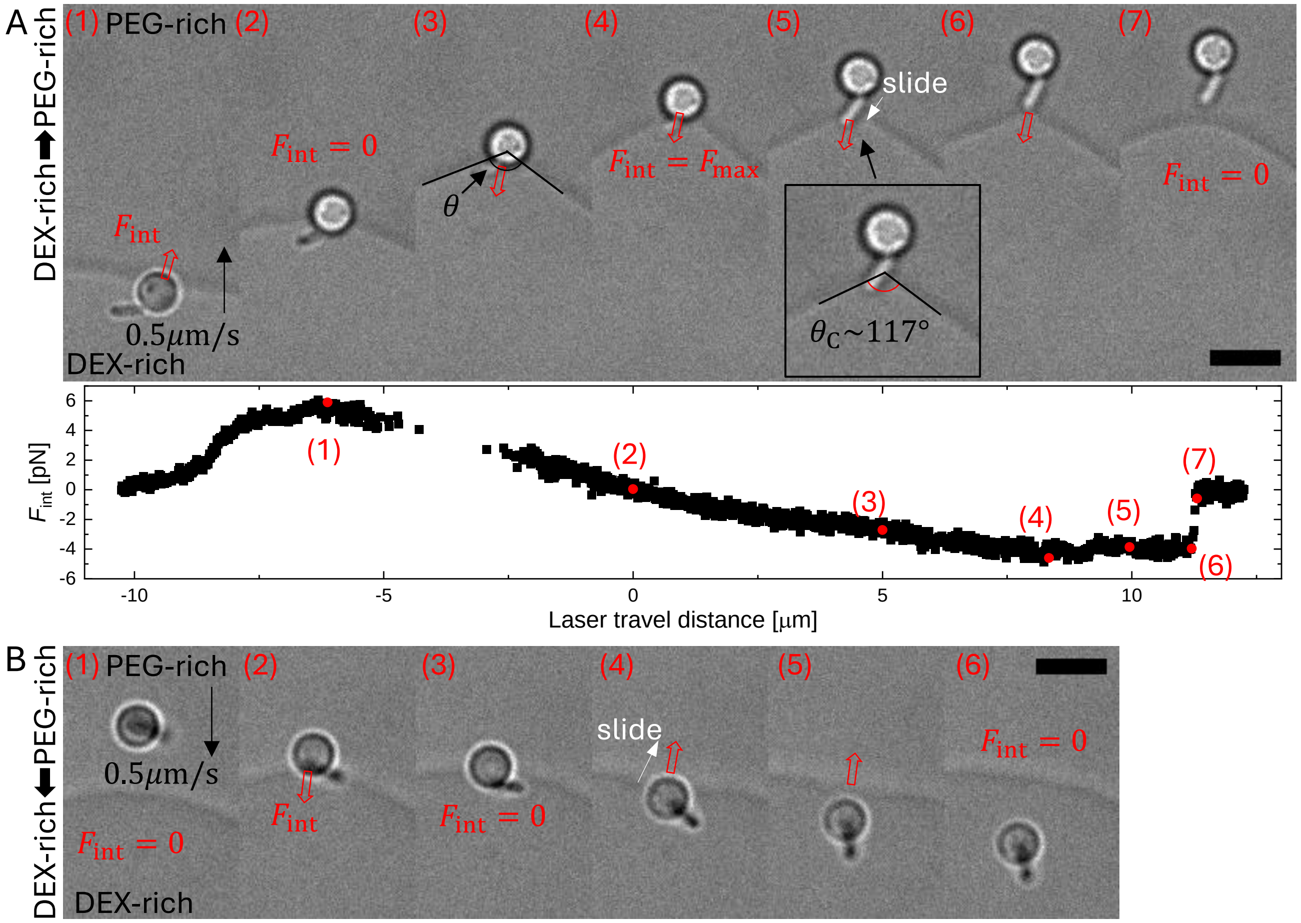


FIG. S5. Optical tweezers experiment snapshots and calibrated force curve. (A) The images are snapshots of the bacterial assembly crossing the PEG-dextran interface from the DEX-rich phase. The force applied on the assembly as measured by the optical tweezers is shown at the bottom. (1) Because of the interaction between the silica bead and the interface, the assembly is pulled forward along the laser's traveling trajectory (0.5 $\mu$m/s, black arrow, same for all snapshots). The force applied by the interface on the assembly, $F_{\text{int}}$, is represented as a red arrow. (2) At the point where $F_{\text{int}} = 0$, the interaction between the bacterial body and the interface begins. (3) $F_{\text{int}}$ increases, but its direction is opposite to the traveling direction. (4) $F_{\text{int}}$ reaches its maximum magnitude, $F_{\text{max}}$. (5) The interface begins sliding (white arrow) over the bacterial body. (6) Finally, the interface releases the assembly. (7) $F_{\text{int}}$ rapidly approaches 0, as the assembly enters the PEG-rich phase completely. (B) The images are snapshots of the bacteria assembly crossing the PEG-dextran interface from PEG-rich phase. (1) The bacteria assembly approaches the interface from the PEG-rich region. (2) Because of the interaction between the bacteria and the interface, now the bacterial part of the assembly is pulled forward along a laser traveling direction. (3) At the point where $F_{\text{int}} = 0$, the interaction between the silica bead and the interface begins. (4) The interface is sliding (white arrow) over the surface of the silica bead. (5) Finally, the interface releases the assembly. (6) $F_{\text{int}}$ rapidly approaches 0, as the assembly enters the DEX-rich phase completely. Scale bar = 5 $\mu$m

The optical tweezers measure the total force applied to the bacteria-colloid assembly. In Fig. S5A, by dividing the measurement into two steps, firstly, in (1) $\sim$ (4), where $F_{\text{int}} < F_{\text{max}}$, the interface deforms and narrowing the $\theta$ because the interface is easier to deform than sliding on the bacterial body, where the force applied by the optical tweezers is weaker than the force from affinity difference.

From (4), when the $F_{\text{int}} = F_{\text{max}}$, the interface stops deforming and starts sliding on the bacterial body, the interface stays at the same position, and $\theta = \theta_C$ became a constant where $\theta_C \sim 117°$. This value reflects the contribution of the deformed interface.

Figure S6, which presents snapshots from Movie S4, shows a swimming bacterium crossing the interface, causing deformation. Due to the higher swimming speed of approximately 30$\mu$m/s, the deformation range is shorter than that

observed in the optical tweezer experiment (Fig. 5A). However, the contribution of these deformations to the forces required to cross the interface is comparable between the swimming bacteria and the optical tweezer experiment, as both exhibit similar contact angles.

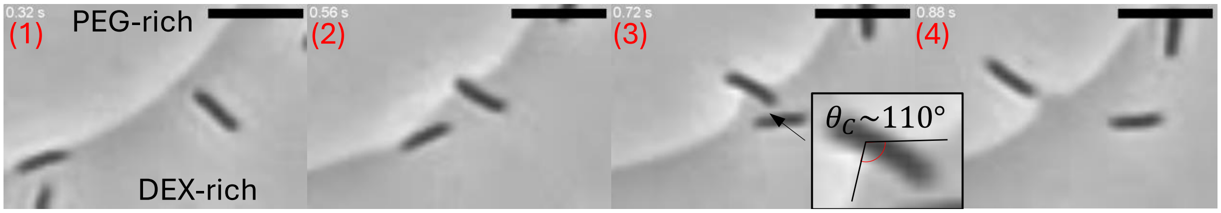


FIG. S6. Experimental images of swimming *Bacillus subtilis* crossing the interface from DEX-rich to PEG-rich. Scale bar = $10\mu$m

## VIII Model

The probability distribution of an active Brownian rod confined in 2-dimensions follows the Smoluchowski equation:

$$\frac{\partial P}{\partial t} + \nabla \cdot \left[\frac{P}{\zeta}\left(\mathbf{F}_{\text{prop}} + \mathbf{F}_{\text{B}} + \mathbf{F}_{\text{ext}}\right)\right] + \frac{\partial}{\partial \theta}\left[\frac{P}{\zeta_R}\left(L_{\text{B}} + L_{\text{ext}}\right)\right] = 0 \tag{S1}$$

where $P(\mathbf{r}, \theta, t)$ is the normalized probability density in the periodic unit cell, $\zeta$ is the translational drag coefficient (which is approximated as a constant independent of particle orientation) and $\zeta_R$ is the rotational drag coefficient. $\mathbf{F}_{\text{prop}} = F_{\text{prop}}[\cos(\theta), \sin(\theta)]^T$, $\mathbf{F}_{\mathbf{B}} = -k_{\text{B}}T\nabla \ln P$, and $\mathbf{F}_{\text{ext}}$ are respectively the active, Brownian, and external forces acting upon the body, and $L_B = -k_{\text{B}}T\frac{\partial \ln P}{\partial \theta}$ and $L_{\text{ext}}$ are the Brownian and external torques.

Ignoring gradients in the $y$ direction, the Smoluchowski equation simplifies to:

$$\frac{\partial P}{\partial t} + \frac{\partial}{\partial x}\left[\frac{P}{\zeta}\left(F_{\text{prop}}\cos(\theta) - k_{\text{B}}T\frac{\partial \ln(P)}{\partial x} - \frac{\partial V}{\partial x}\right)\right] + \frac{\partial}{\partial \theta}\left[P\left(-\frac{1}{\tau_R}\frac{\partial \ln(P)}{\partial \theta} - \frac{1}{\zeta_R}\frac{\partial V}{\partial \theta}\right)\right] = 0, \tag{S2}$$

where $\tau_R$ is the reorientation time.

To study the partitioning between two phases, we model a repeating lamellar phase using a 1-D periodic potential of strength $A$ and wavelength $L$: $\phi(x) = -A\tanh\left[\frac{L}{2\pi\delta}\cos\left(\frac{2\pi x}{L}\right)\right]$ with $\delta \ll L$ to approximate a square wave. For a finite-sized body described by density $\rho(\mathbf{s})$, the potential energy $V$ of the body is given by the convolution $V(\mathbf{r}, \theta) = \int \phi(\mathbf{r} - \mathbf{s})\rho(\mathbf{s})d\mathbf{s}$. We compute the convolution as a product in Fourier space

$$\hat{V}_n(\theta) = \hat{\phi}_n\hat{\rho}_n(\theta). \tag{S3}$$

The $n$-th Fourier coefficient of the line density $\hat{\rho}_n$ can be derived analytically [? ], allowing us to determine an expression for the center of mass potential directly.

$$V(x, \theta) = \sum_n \hat{\phi}_n e^{i2\pi k_n x}\text{sinc}\left(\pi\ell_{\text{bact}}k_n\cos(\theta)\right). \tag{S4}$$

The wavevector is defined as $k_n = \frac{n}{L_x}$, and the bacteria length is $\ell_{\text{bact}}$. This method converges rapidly for periodic potentials with a low-wavenumber power spectrum. The $\text{sinc}(\pi\ell_{\text{bact}}k_n\cos(\theta))$ term comes from the Fourier transform of the segment density for a rod and couples the orientation of the bacterium to the potential energy. We solve Eq. S2 at steady state using spectral methods implemented in the spectral PDE solver Dedalus [? ].

## IX Parameters obtained from the experiments: Runlength, Domain radius, and propulsion force

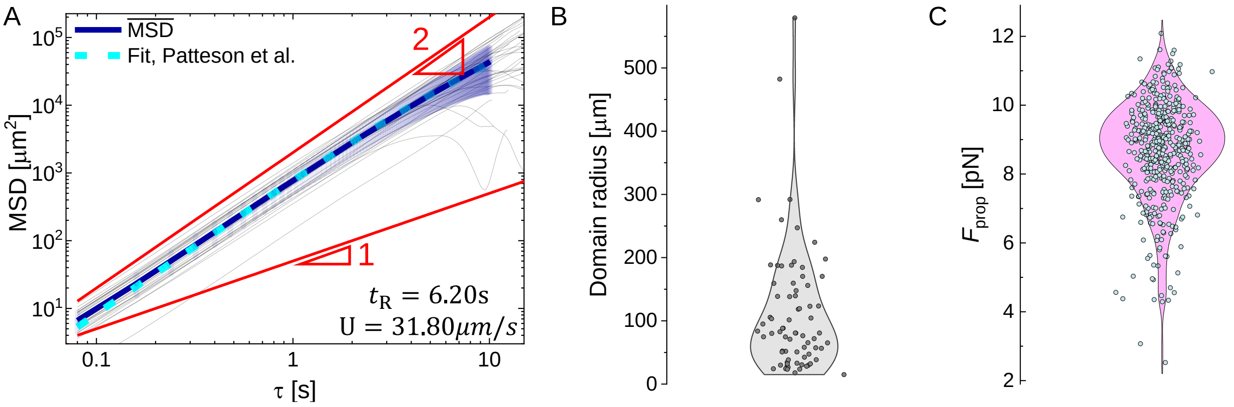


FIG. S7. Experimental data of *B. subtilis* and the sample area. (A) The mean square displacement of *B.subtilis* in ATPS (where dextran concentration is 3.2wt/wt%). The navy line indicates the averaged MSD until $\tau$ = 10s with the standard deviation plotted as a shadow and the cyan dashed line is the fitting line by the run-and-tumble model. Two red lines are reference slopes of 1 and 2. The background lines are the raw data obtained with individual *B. subtilis* cells. (B) The radius of the sampled PEG-rich domain. The area of the domain was estimated and, assumed to be circular, and used to calculate the average radius. (C) Propulsion force of *B. subtilis* obtained by multiplying its speed with the drag coefficient of a prolate ellipsoid ([**?** ], the body length and the diameter of the bacterium's body were considered as the major and minor axes, respectively) in the DEX-rich phase (from ATPS prepared with3.2 wt/wt% dextran).

We collect 37 trajectories of bacteria swimming the quasi-2D ATPS longer than 10s, to calculate the MSD as in Fig. S7A. The navy line is the average MSD trajectory of 10s and the run-and-tumble model fits the data as the dashed line. Run-and-tumble model for swimming bacteria in polymeric solution [**?** ] which contains active diffusion coefficient, $D_{\mathrm{act}}$, is

$$MSD(\Delta t) = 4D_{\mathrm{act}}\Delta t(1 - e^{-\frac{\Delta t}{t_{\mathrm{R}}}}) \tag{S5}$$

and gives $D_{\mathrm{act}} = 1295\mu\mathrm{m}^2/s$ and $t_{\mathrm{R}} = 6.20$s where the average run length ($l_{\mathrm{run}} = t_{\mathrm{R}}U$) is 186.68$\mu$m.

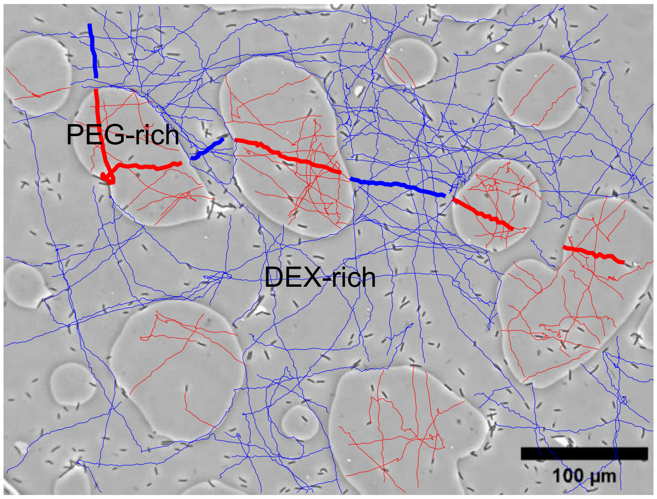


FIG. S8. Experimental data of *B. subtilis* swimming trajectories in ATPS. The red lines correspond to the trajectories of bacteria swimming in the PEG-rich phase, and the blue lines correspond to the ones in the DEX-rich phase(from ATPS prepared with 3.2 wt/wt% dextran).

We estimate the mean square displacement (MSD) from each trajectory. Fitting the MSD with $\mathrm{MSD}(\Delta t) = 4D_{\mathrm{act}}\Delta t(1 - e^{-\frac{\Delta t}{t_{\mathrm{R}}}})$, we get the average reorientation times $t_{R,\mathrm{DEX-rich}} = 4.6 \pm 0.1$ s and $t_{R,\mathrm{PEG-rich}} = 1.7 \pm 0.1$ s,

which correspond to the average run lengths ($l_{\rm run} = t_R U$) is $59 \pm 15$ $\mu$m in the PEG-rich phase and $141 \pm 32$ $\mu$m in the DEX-rich phase. Although the considerably shorter run length in the PEG-rich phase seemingly hints at the chemotactic scenario, we find the domain size of the PEG-rich phases, *i.e.*, the dispersed island in the Fig. S8, is comparable to the run length in the PEG-rich phase. Namely, the domain size is responsible for the shorter run length in the PEG-rich phase because the bacterial motion is affected at the interface. Therefore, we cannot judge the chemotaxis from the estimated run length in each phase.

## X Sensitivity analysis

In the considered experimental system, there are seven parameters: the maximum force to cross the interface $F_{\rm max}$, bacterial propulsion force $F_{\rm prop}$, bacterium length $l$, reorientation time $\tau_{\rm R}$, effective interfacial width $\delta$, domain size $L$, and thermal diffusivity $D_{\rm T}$. From these, our model is described with five nondimensionalized parameters: the ratio of the maximum interface restoring force to the propulsion force $F_{\rm max}/F_{\rm prop}$, the ratio of propulsion force relative to thermal energy $(F_{\rm prop}L)/k_{\rm B}T$, the ratio of thermal diffusivity relative to the reorientation time $L^2\zeta/(\tau_R k_{\rm B}T)$, the scaled bacteria length $\ell_{\rm bact}/L$, and the scaled effective interface width $\delta/L$.

We have experimentally measured the parameters except $\delta$ and $tau_{\rm R}$ which are challenged to estimate exact values. So we found those parameters by fitting and the results have multiple parameter sets of $\delta$ and $\tau_{\rm R}$ that show identical partitioning. However, how each parameter affects the partitioning can not be understood by fitting. Thus we alternatively performed a sensitivity analysis of how theoretical results would change by parameter variations.

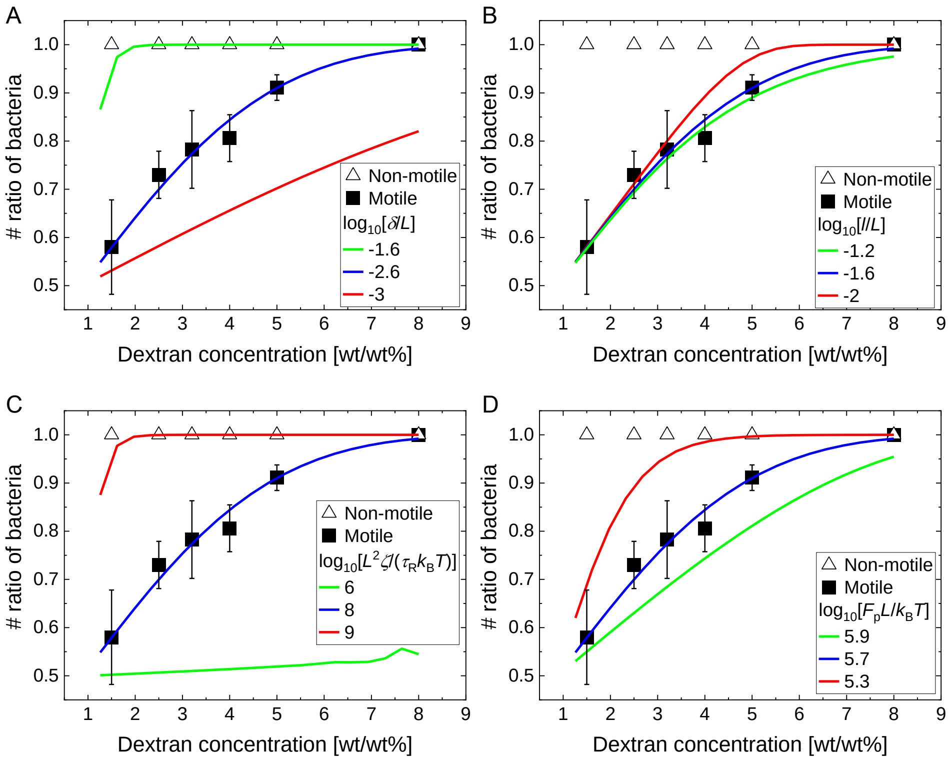


FIG. S9. Sensitivity analysis of each parameter. Each parameters are initially set as $\log[\delta/L] = -2.6$, $\log[l/L] = -1.6$, $\log[L^2/\tau_{\rm R} D_T] = 8$, and $\log[F_{\rm p}L/k_{\rm B}T] = 5.7$. In all cases (A-D), the blue line represents the result presented in Fig. 2 of the main text. The green and red lines indicate the upper and lower boundaries of experimental measurements (B and D) and the expected bounds within the realistic region (A and C), respectively.

As shown in Fig. S9, our prediction is extremely sensitive in two parameters $\delta$ and $\tau_{\rm R}$ (see Fig. S9A and C). In all cases Fig. S9(A-D), the blue line represents the result presented in Fig. 2 of the main text. The green and red lines correspond to the upper and lower boundaries of either the realistic region estimation (A, and C) or experimental measurements (B, and D). Specifically for Fig. S9A, the green line indicates when effective interfacial width is $\delta = 5.0$ $\mu$m and the red line for $\delta = 0.2$ $\mu$m where the blue line is when $\delta = 0.5$ $\mu$m. For Fig. S9C, the green curve is when $\tau_{\rm R} = 1.4$ s and the red curve is when $\tau_{\rm R} = 0.0014$ s where the blue line indicates $\tau_{\rm R} = 0.014$ s For

Fig. S9B and D which are based on the experimental observation the green line in Fig. S9B indicates when bacterium body length is $l = 12.6$ $\mu$m and the red line for $l = 2.0$ $\mu$m where the blue line is when $l = 5.0$ $\mu$m. For Fig. S9D, based on the measurement in Fig. S7C, the green curve is when $F_{\text{prop}} = 15.9$ pN and the red curve is when $F_{\text{prop}} = 4.0$ pN where the blue line indicates $F_{\text{prop}} = 10.0$ pN. These estimations in (A-D) are, for simplicity, we consider the $L = 200$ $\mu$m as a fixed number.
